# Supplementary material for: RAGUEL: Recourse-Aware Group Unfairness Elimination
Source: arXiv:2208.14175 source file (2022-08-30)
Supplement: Supplementary file 1 [file appendix.tex]

\section{Data pre-processing}
\label{app:attr}

All code and data used in this paper will be made publicly available.

\begin{table}[h]
\caption{Modified attribute columns for German Credit dataset}
\label{tab:1}
\begin{tabular}{cc}
\toprule
\textbf{Attribute} & \textbf{Value Type} \\
\midrule
Gender & binary \\
Single & binary \\
Age & numerical \\
LoanDuration & binary \\
LoanPurpose & categorical \\
LoanAmount & numerical \\
LoanRateAsPercentOfIncome & numerical \\
HasCheckingAccount & binary \\
HasSavingsAccount & binary \\
NumberOfExistingLoans & numerical \\
NumberOfLiableIndividuals & numerical \\ 
HasOtherDebtor & binary \\
LengthOfEmployment & numerical \\
JobType & categorical \\
Unemployed & binary \\
RentsOwnsHome & binary \\
YearsInCurrentHome & numerical \\
HasTelephone & binary \\
\bottomrule
\end{tabular}
\end{table}

\begin{table}[h]
\caption{Modified attribute columns for DC3 dataset}
\label{tab:1}
\begin{tabular}{cc}
\toprule
\textbf{Attribute} & \textbf{Value Type} \\
\midrule
Married & binary \\
Single & binary \\
EducationLevel & categorical \\
MaxBillAmountOverLast6Months & numerical \\
MaxPaymentAmountOverLast6Months & numerical \\
MonthsWithZeroBalanceOverLast6Months & numerical \\
MonthsWithLowSpendingOverLast6Months & numerical \\
MonthsWithHighSpendingOverLast6Months & numerical \\
MostRecentBillAmount & numerical \\
MostRecentPaymentAmount & numerical \\
\bottomrule
\end{tabular}
\end{table}
